# Supplementary material for: Entropy-driven Sampling and Training Scheme for Conditional Diffusion Generation
Source: arXiv:2206.11474 source file (2022-09-20)
Supplement: Supplementary file 1 [file ablations_grad_norm.tex]

\begin{figure}[th]
     \centering
     \includegraphics[width=0.45\textwidth]{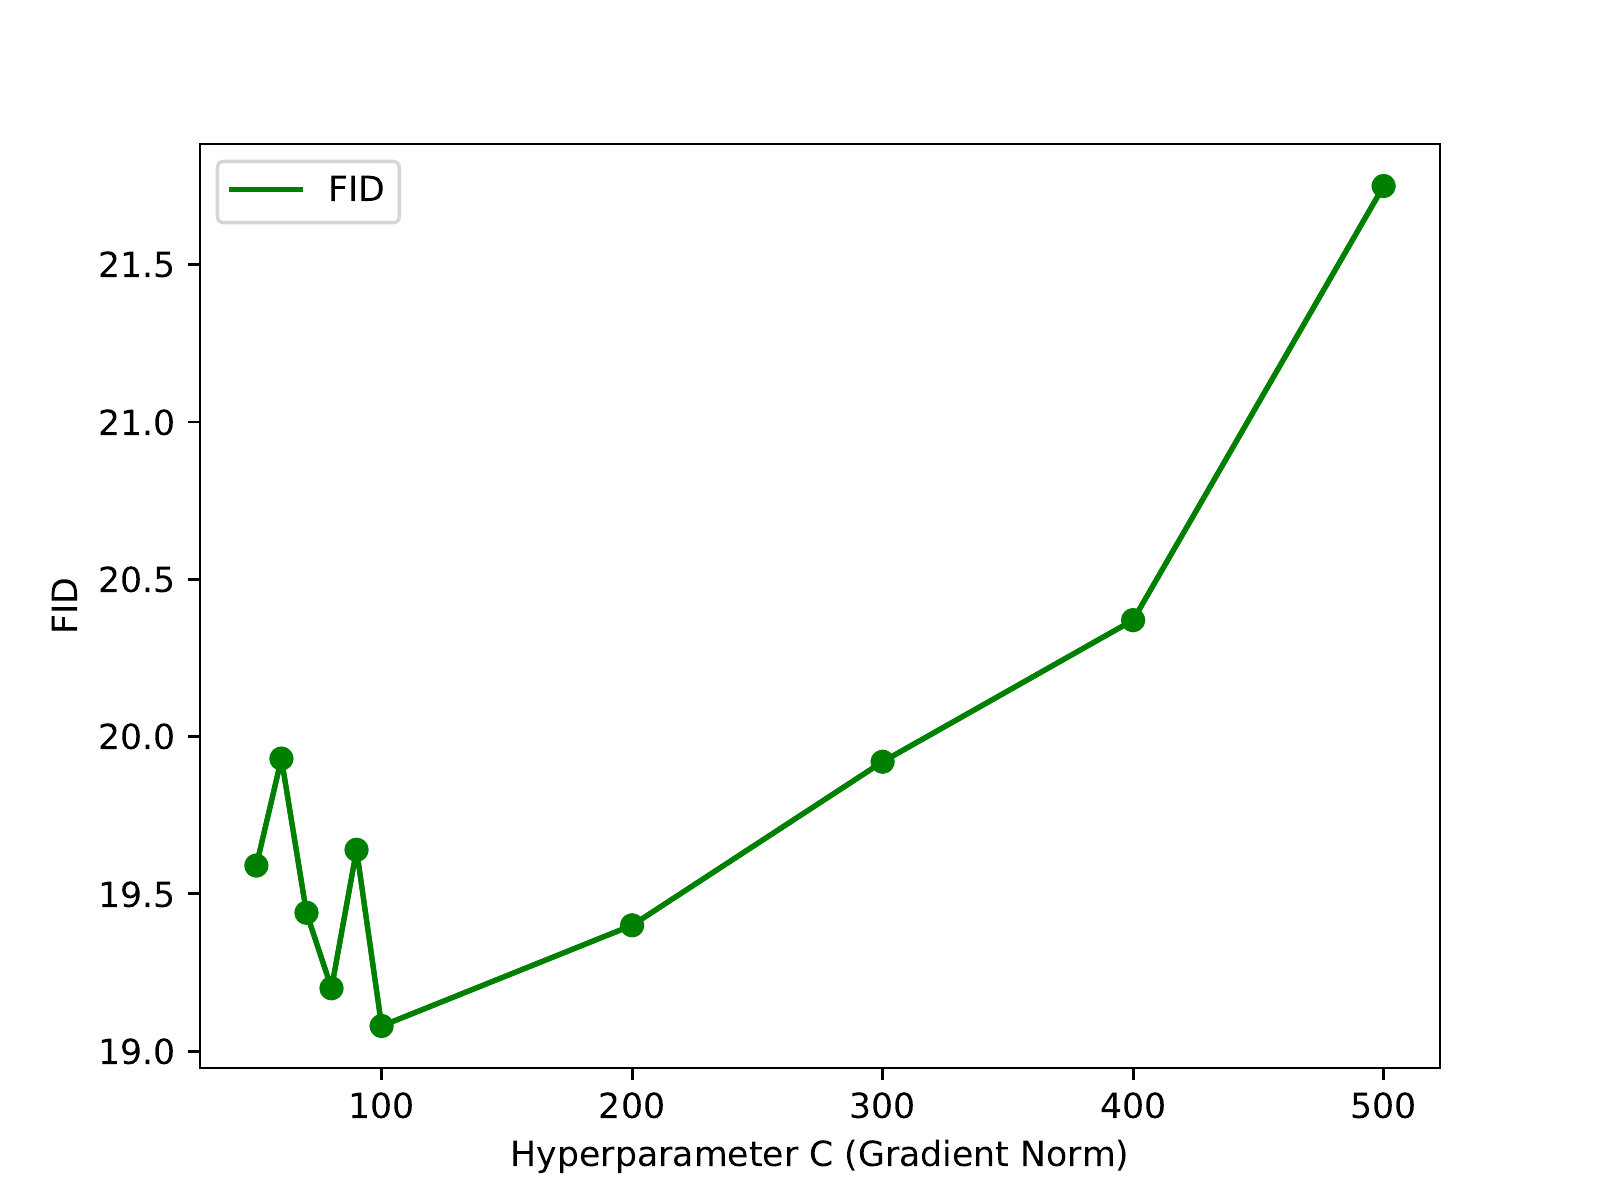}
     \caption{Ablation of Gradient Norm}
     \label{fig:compare_0}
    \caption{The curve plot of optimal hyperparameter $C$ based on 5k images for Gradient Norm method.} \label{fig:grad_ablation}
\end{figure}
