# Supplementary material for: Entropy-driven Sampling and Training Scheme for Conditional Diffusion Generation
Source: arXiv:2206.11474 source file (2022-09-20)
Supplement: Supplementary file 2 [file ablations_time_constant.tex]

\begin{figure}[th]
     \centering
     \begin{subfigure}[b]{0.45\textwidth}
         \centering
         \includegraphics[width=\textwidth]{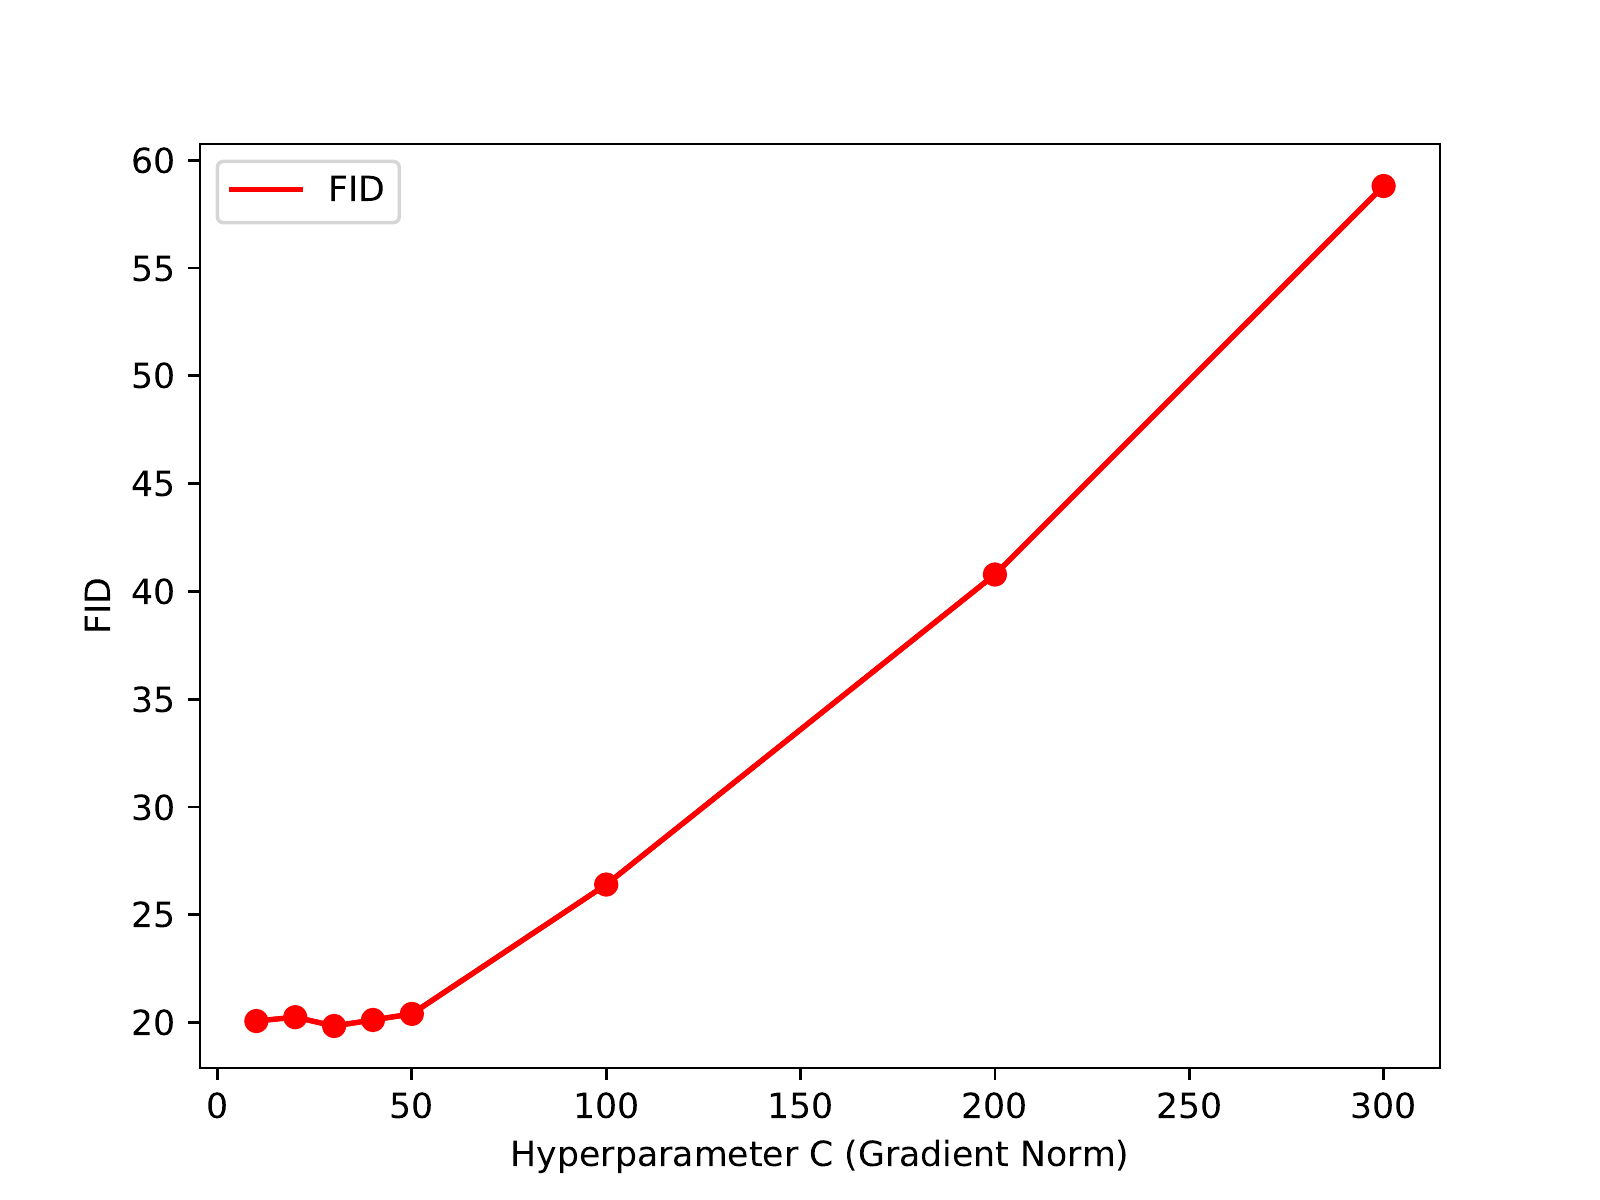}
         \caption{Ablation of Constant(range 0-700)}
         \label{fig:compare_0}
     \end{subfigure}
    %  \hfill
     \begin{subfigure}[b]{0.45\textwidth}
         \centering
         \includegraphics[width=\textwidth]{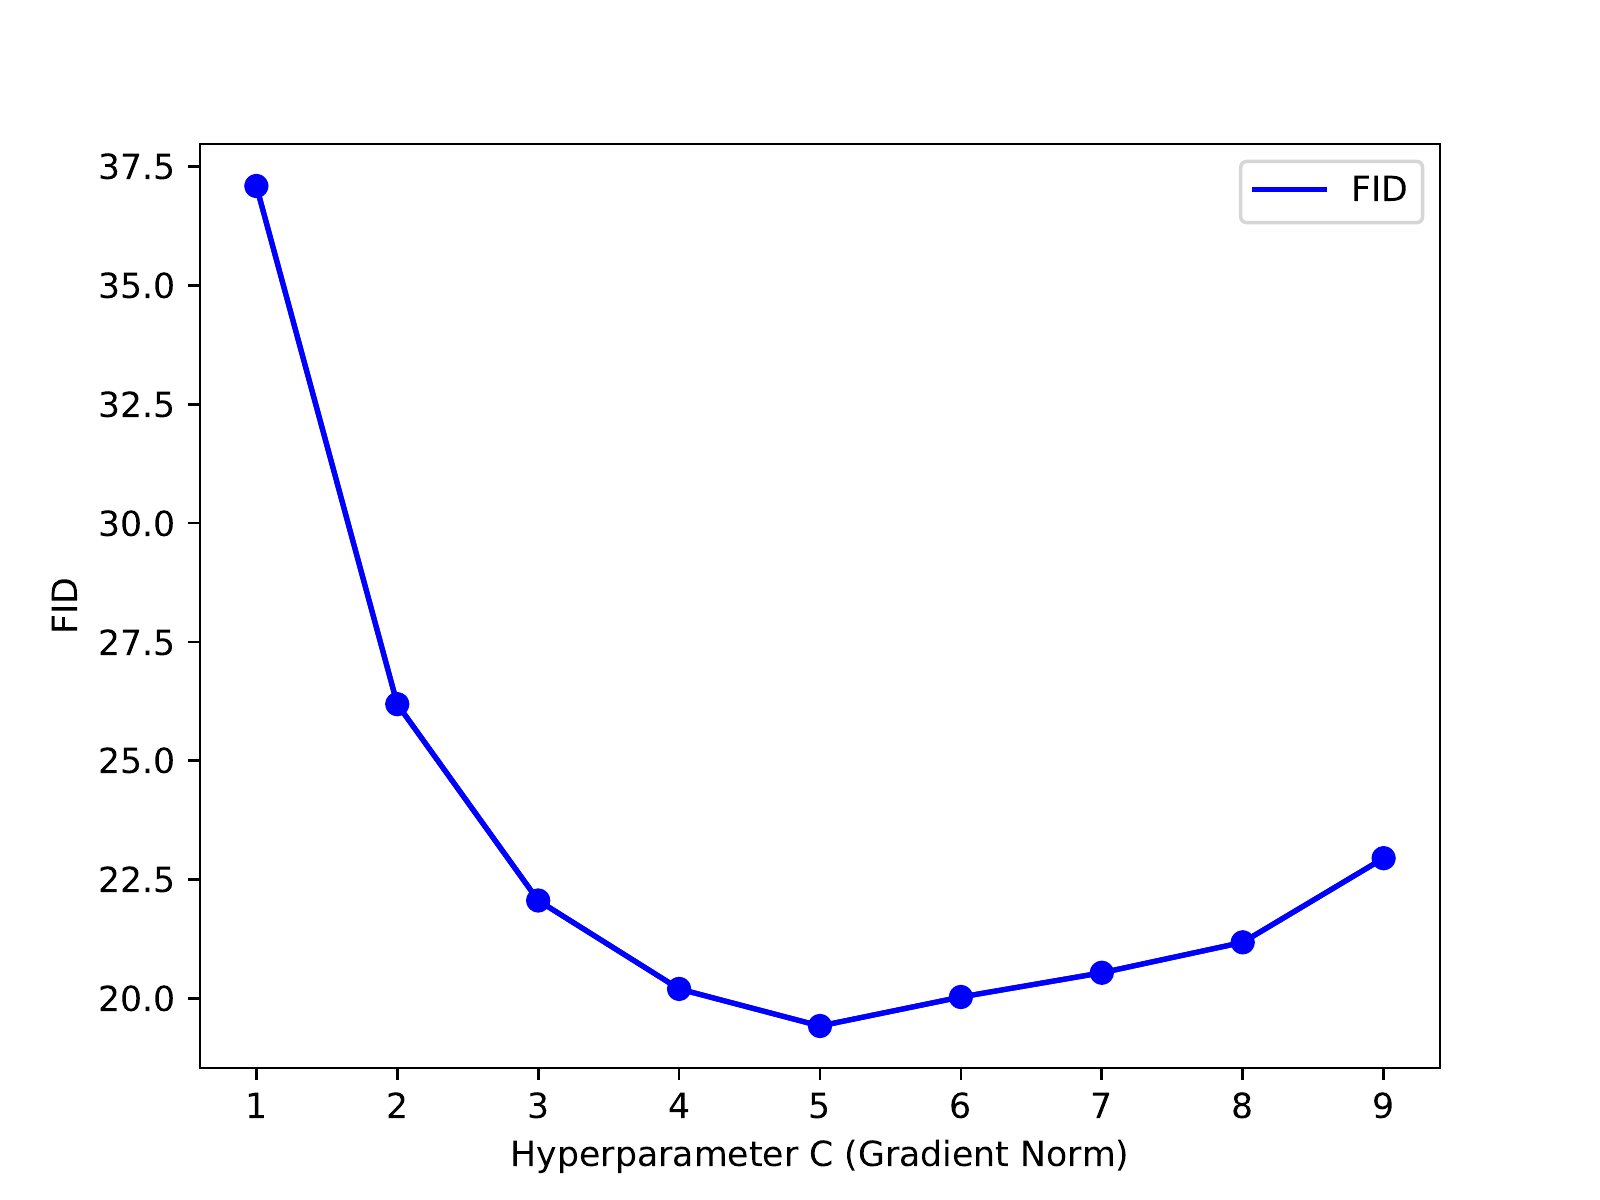}
         \caption{Ablation of Time-aware}
         \label{fig:compare_1}
     \end{subfigure}
     
    %  \begin{subfigure}[b]{0.3\textwidth}
    %      \centering
    %      \includegraphics[width=\textwidth]{supplement/ablations_time.png}
    %      \caption{Ablation of Time-aware}
    %      \label{fig:compare_1}
    %  \end{subfigure}
        % \includegraphics[width=0.5\textwidth]{supplement/ablations_time.png}
    \caption{The curve plot of optimal EDS hyperparameter $C$ based on 5000 images evaluated with FID for Constant and Time-aware methods separately.} 
    \label{fig:time_const_ablation}
\end{figure}
