# Supplementary material for: Entropy-driven Sampling and Training Scheme for Conditional Diffusion Generation
Source: arXiv:2206.11474 source file (2022-09-20)
Supplement: Supplementary file 5 [file ablation_sample.tex]

\begin{figure}[th]
    \begin{center}
        \includegraphics[width=\textwidth]{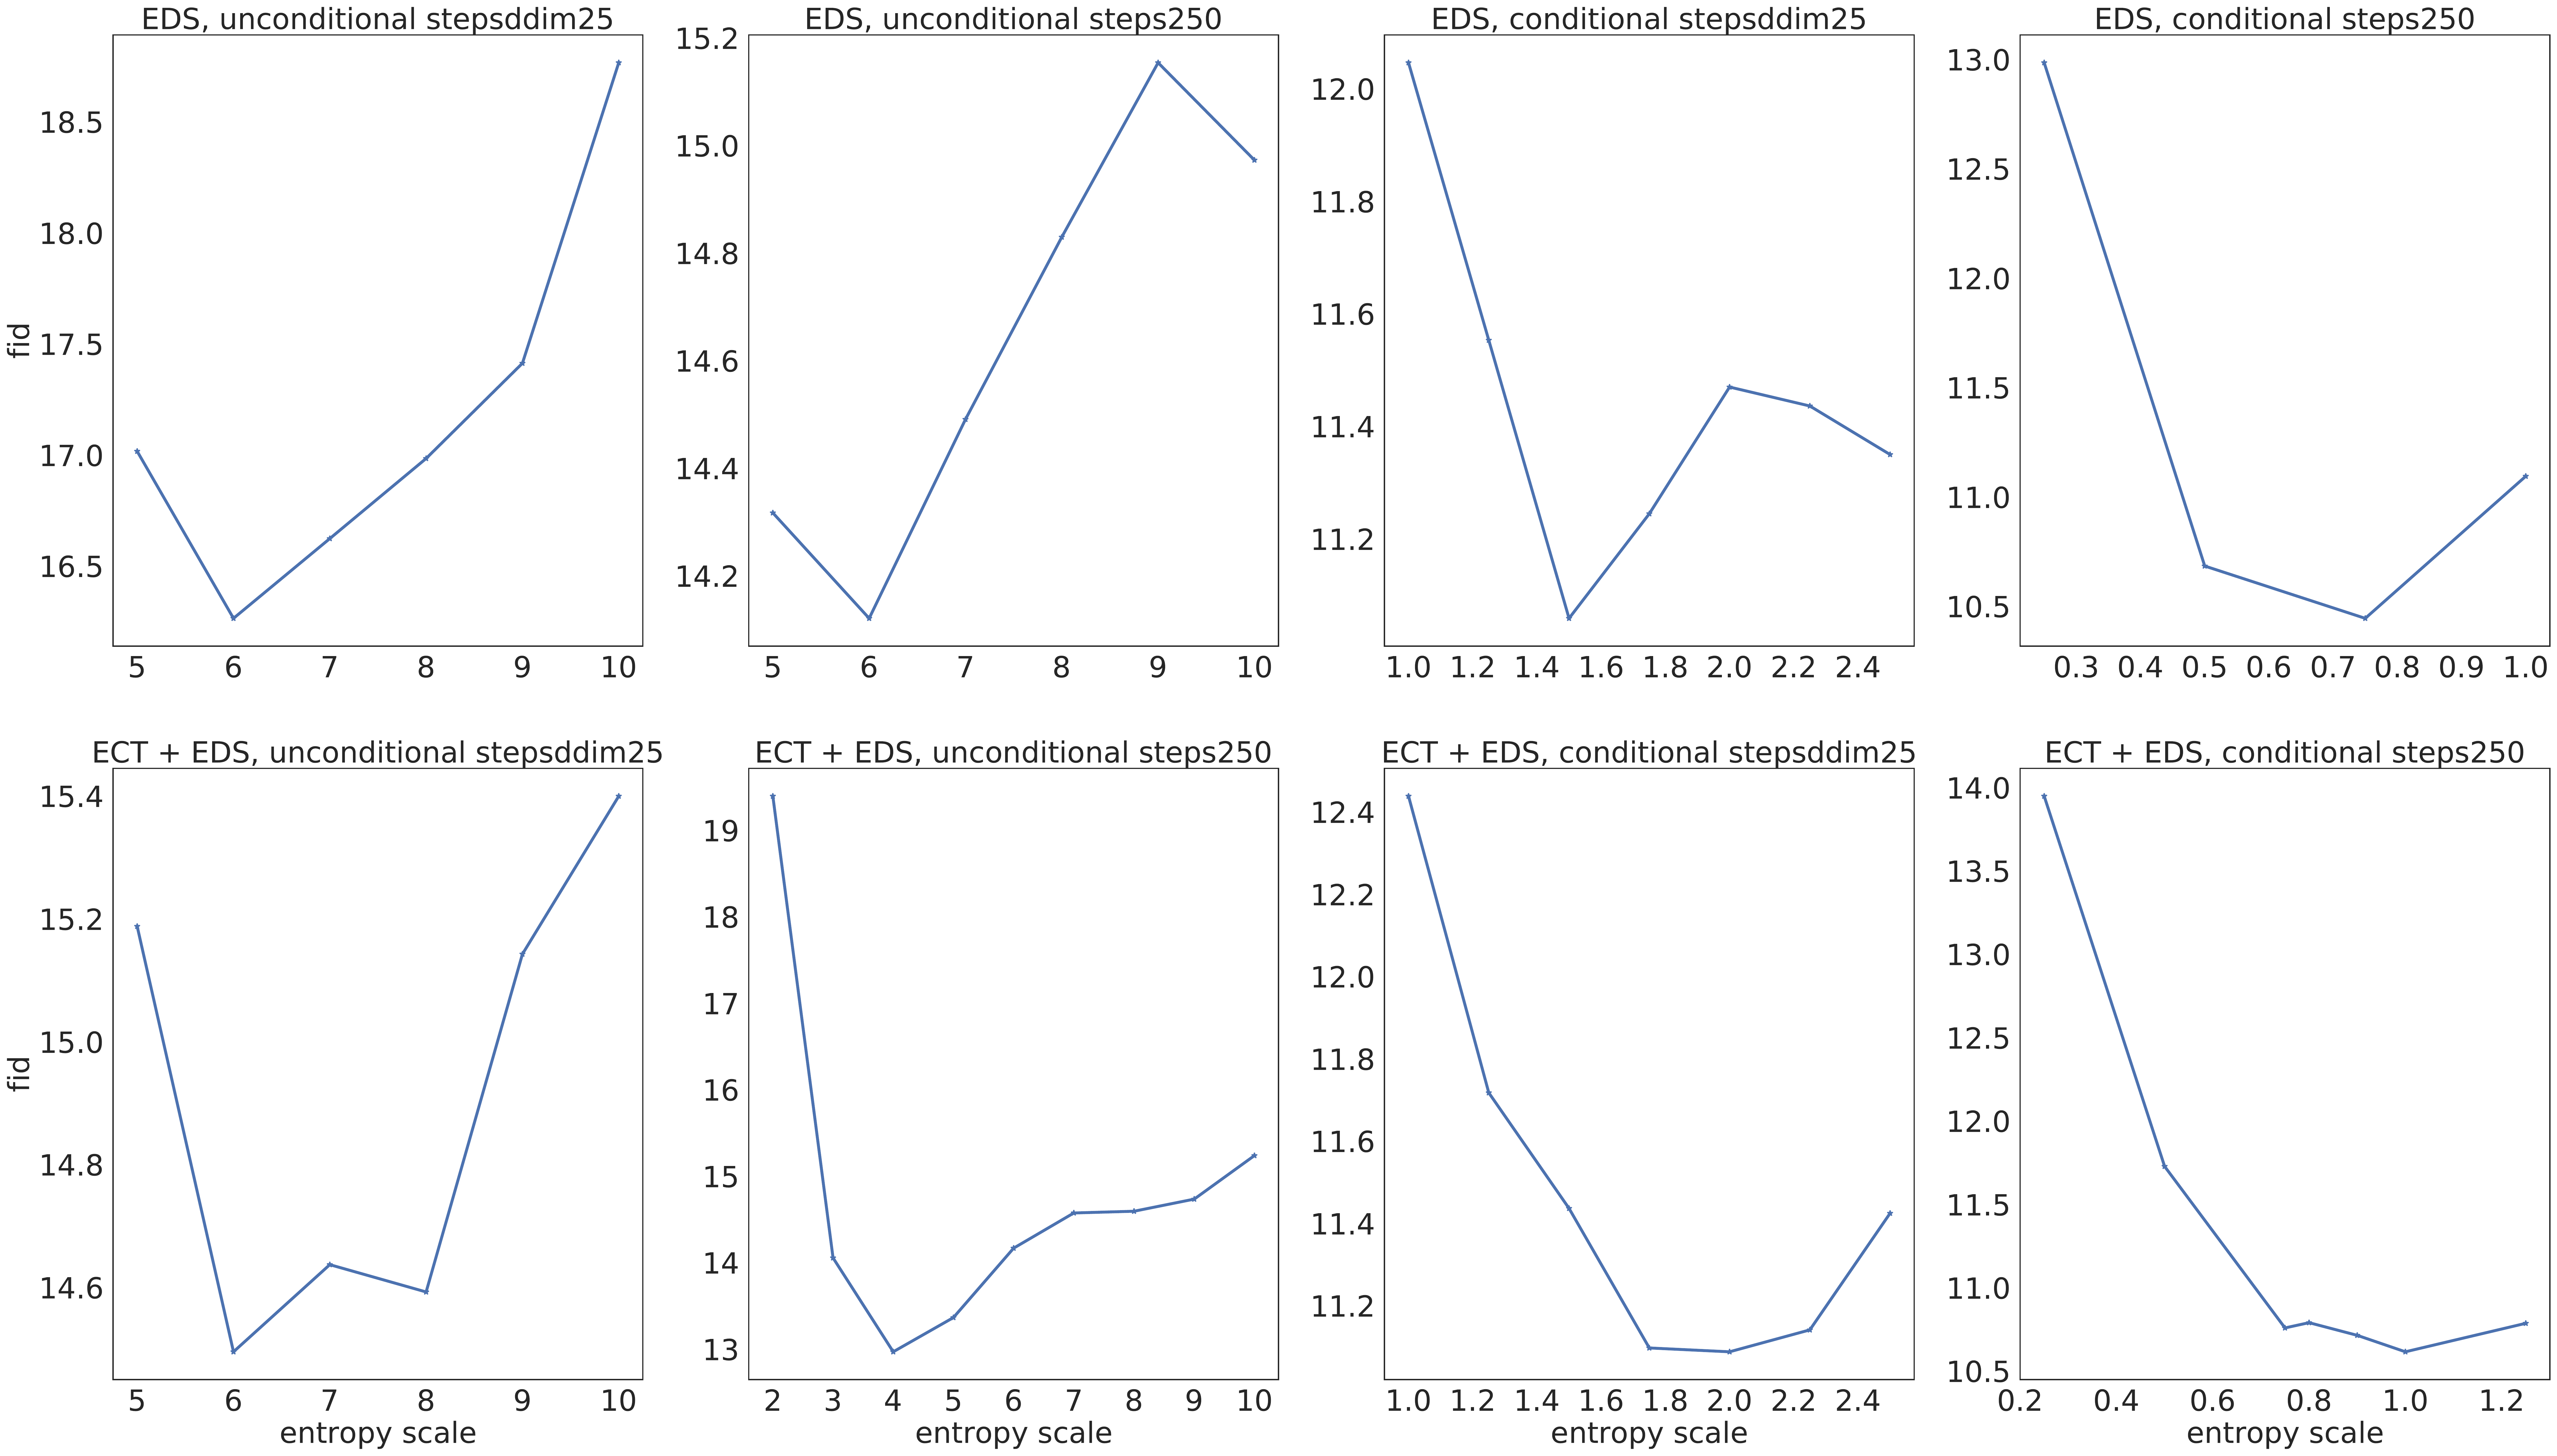}
    \end{center}
    \caption{The curve plot of optimal EDS hyperparameter $\gamma$ based on 5k images evaluated with FID.} 
    \label{fig:class_scale}
\end{figure}
